# Supplementary material for: Sound-Word2Vec: Learning Word Representations Grounded in Sounds
Source: arXiv:1703.01720 source file (2017-08-29)
Supplement: Supplementary file 1 [file appendix.tex]

\noindent \textbf{Feature Space for Clustering.} The freesound database \cite{freesound} provides multiple precomputed sound descriptors that can be downloaded for each sound. 
The feature vector for a sound is the \emph{concatenation of the mean and variance} of the following audio descriptors: \\
\begin{compactenum}
\item Mel-Frequency Cepstral Co-efficients: \ak{This feature represents the short-term power spectrum of an audio and closely approximates the response of the human auditory system -- computed as given in \cite{ganchev2005comparative}.}
\item Spectral Contrast: It is the magnitude difference in the peaks and valleys of the spectrum -- computed according to \cite{akkermans2009shape}.
\item Dissonance: It measures the perceptual roughness of the sound \cite{plomp1965tonal}.
\item Zero-crossing Rate: It is the number of sign changes between consecutive signal values divided by the total number of values. 
        A higher zero-crossing rate indicates the presence of noise.
    \item Spectral Spread: This feature is the concatenation of the $k$-order moments of the spectrum, where $k \in \{0,1,2,3,4\}$.
    \item Pitch Salience: This feature helps disciminate between musical and non-musical tones. 
        While, pure tones and unpitched sounds have values near 0, musical sounds containing harmonics have higher values \cite{ricard2004towards}.
    \end{compactenum}
    Of all the pre-computed features available on the freesound database, we use those that exhibit significant variance across the sounds in the dataset \ie descriptors that are nearly the same for most sounds do not contain significant discriminatory information and hence, are discarded.
    \\ \\
    \textbf{Comparison with \cite{kiela_emnlp15}}
    As against using embeddings trained by us, we use the pre-trained vectors released by the authors. 
    These embeddings achieve a recall@100 of 27.18 (as against 28.67 achieved by sound-word2vec) on the text-based sound retrieval task and a mean rank of 45.4 (as compared to 34.6 got by our method) on the task of foley-sound discovery. 
    Further, as reported in the paper \cite{kiela_emnlp15}, they achieve a score of 0.662 and 0.345 on the AMEN and ASLex datasets respectively (as against 0.674 and 0.391 respectively for sound-word2vec). \\ \\
    Using these pre-trained vectors does not result in a fair comparison between the methods as they are not trained on the exact same data and hence, include them in the supplementary.
